# Supplementary material for: Intelligent Monitoring Framework for Cloud Services: A Data-Driven Approach
Source: arXiv:2403.07927 source file (2024-02-29)
Supplement: Supplementary file 1 [file Appendix.tex]

\clearpage % Start the appendix on a new page
\onecolumn % Use the entire page width for the appendix

\appendix

\section{Ablation Study}
In this ablation study, we investigate the impact of different features on the performance of a binary classification model for various resource classes. The features under consideration include upstream dependency, components of the service, and a combination of both.
\subsection{Methodology}
\subsubsection{Dataset Creation}
\begin{itemize}
    \item Construct a binary matrix with services as rows and service features and resource classes as columns.
    \item Divide the dataset into two parts:
    \begin{itemize}
        \item dataset\_train (80\%): Retain all columns with actual values.
        \item dataset\_test (20\%): Preserve columns, excluding resource classes, for services in the test set.
    \end{itemize}
    \item Create dataset\_combined by merging dataset\_train and dataset\_test.
\end{itemize}
\subsubsection{Model Training}
\begin{itemize}
    \item Train a collaborative filtering model using Singular Value Decomposition on dataset\_combined.
\end{itemize}
\subsubsection{Model Evaluation}
\begin{itemize}
    \item Assess the model on dataset\_test by predicting missing resource classes. Evaluate quantitative metrics.
\end{itemize}
\subsubsection{Results Analysis}
\begin{itemize}
    \item Analyze the predicted resource classes and compare them to the actual values.
    \item Examine the overall performance of the collaborative filtering model in recommending resource classes for services.
\end{itemize}
\subsection{Experiment Setup}
We focused on several resource classes, including storage, API, none-of-the-above, dependency, service level, ram-memory, cache-memory, CPU, certificate, container, and compute cluster. For each resource class, we conducted experiments with three feature scenarios: upstream dependency only, components only, and both.
\subsection{Results}
Below are the AUC scores for each resource class in the three feature scenarios:
\begin{table}[h!]
\caption{AUC Scores for different resource classes}
\centering
\resizebox{0.5\textwidth}{!}{%
% \begin{tabular}{|c|p{2.4cm}|p{2.4cm}|p{2.4cm}|} 
\begin{tabular}{|c|c|c|c|} 
 \hline
 Resource Class & Upstream Dependency Only & Components Only & Both Features \\
 \hline\hline
 Service level & \begin{tabular}{@{}c@{}}0.47 \end{tabular} & \begin{tabular}{@{}c@{}} 0.82\end{tabular} & \begin{tabular}{@{}c@{}}0.39 \end{tabular}\\
 \hline
 API & \begin{tabular}{@{}c@{}}0.58 \end{tabular} & \begin{tabular}{@{}c@{}}0.67 \end{tabular} & \begin{tabular}{@{}c@{}}0.62 \end{tabular}\\
 \hline
 CPU & \begin{tabular}{@{}c@{}}0.57 \end{tabular} & \begin{tabular}{@{}c@{}}0.68 \end{tabular} & \begin{tabular}{@{}c@{}}0.64 \end{tabular}\\
 \hline
 Container & \begin{tabular}{@{}c@{}}0.77 \end{tabular} & \begin{tabular}{@{}c@{}}0.70 \end{tabular} & \begin{tabular}{@{}c@{}}0.71 \end{tabular}\\
 \hline
 Dependency & \begin{tabular}{@{}c@{}}0.35 \end{tabular} & \begin{tabular}{@{}c@{}} 0.79\end{tabular} & \begin{tabular}{@{}c@{}}0.64 \end{tabular}\\
 \hline
 Compute cluster & \begin{tabular}{@{}c@{}}0.62 \end{tabular} & \begin{tabular}{@{}c@{}}0.76 \end{tabular} & \begin{tabular}{@{}c@{}}0.68 \end{tabular}\\
 \hline
 Storage & \begin{tabular}{@{}c@{}}0.58 \end{tabular} & \begin{tabular}{@{}c@{}} 0.69\end{tabular} & \begin{tabular}{@{}c@{}}0.62 \end{tabular}\\
 \hline
 Ram-memory & \begin{tabular}{@{}c@{}}0.44 \end{tabular} & \begin{tabular}{@{}c@{}}0.64 \end{tabular} & \begin{tabular}{@{}c@{}}0.60 \end{tabular}\\
 \hline
 Certificate & \begin{tabular}{@{}c@{}}0.40 \end{tabular} & \begin{tabular}{@{}c@{}}0.70 \end{tabular} & \begin{tabular}{@{}c@{}}0.24 \end{tabular}\\
 \hline
 Cache-memory & \begin{tabular}{@{}c@{}}0.66 \end{tabular} & \begin{tabular}{@{}c@{}}0.83 \end{tabular} & \begin{tabular}{@{}c@{}}0.67 \end{tabular}\\
 \hline
 None-of-the-above & \begin{tabular}{@{}c@{}}0.47 \end{tabular} & \begin{tabular}{@{}c@{}}0.89 \end{tabular} & \begin{tabular}{@{}c@{}}0.55 \end{tabular}\\
 \hline
\end{tabular}
}
\label{tab:finalrecco}
\end{table}

% The aim is to provide a detailed analysis of the model's discriminative capabilities across various aspects of our system.
% \begin{figure}[hbt!]
%     \centering
%     \includegraphics[scale=0.25]{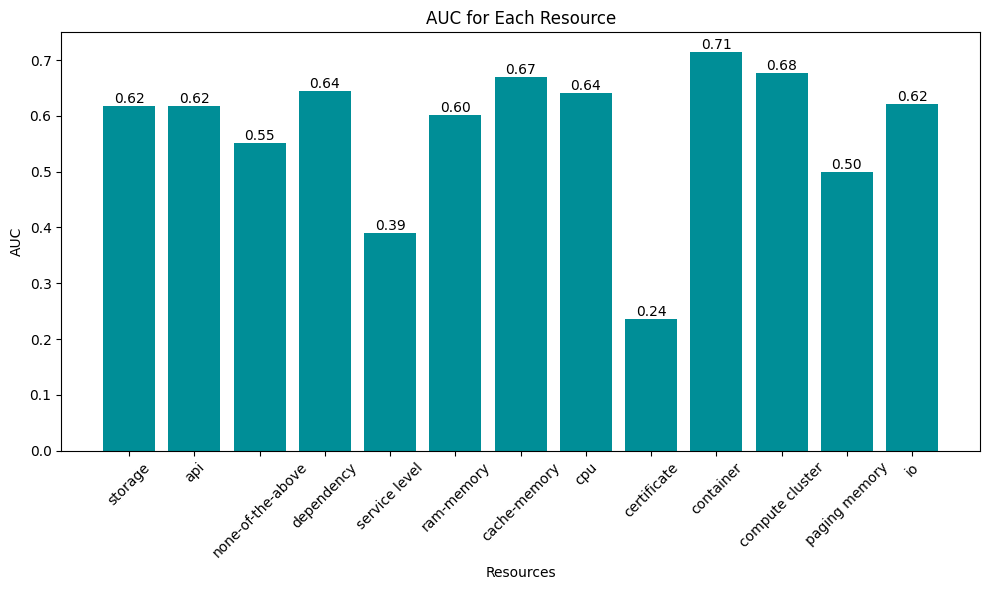}
%     \caption{AUC values for different resource classes}
%     \label{fig:auc}
% \end{figure}
\subsection{Analysis}
The observed AUC scores across different feature scenarios unveil interesting insights into the behavior of the binary classification model for various resource classes. In the case of the "Storage" class, the highest AUC score of 0.69 was achieved when only dimensions were considered. Surprisingly, the combined inclusion of upstream dependency and dimensions did not yield the highest AUC in this case, emphasizing the unique sensitivity of the model to individual features within this resource class.\\

Conversely, in the "API" resource class, AUC scores remained relatively consistent between scenarios of upstream dependency only (0.58) and dimensions only (0.67). This suggests that, for API, either feature independently provides sufficient discriminatory power for effective classification.

\subsection{Conclusion}
In conclusion, our ablation study provides nuanced insights into the impact of feature selection on the binary classification model's performance across diverse resource classes. The unexpected high AUC score of 0.89 for the "None-of-the-Above" class when only dimensions were considered emphasizes the critical role of dimensions in effective classification within this broad category. \\

These findings underscore the necessity for a tailored approach to feature engineering, recognizing the unique characteristics of each resource class. The insights gained from this study pave the way for future research, urging exploration into additional features or refinement of existing ones to enhance the model's discriminative ability. 
% \newpage
% \section*{Appendix}
% Here we will present the scope of our work and experiment results. 
% \subsection*{A.1}
% In this section, we conduct an ablation study to evaluate the performance of our binary classification model on individual resource classes. The aim is to provide a detailed analysis of the model's discriminative capabilities across various aspects of our system.
% \normalsize
